# Supplementary material for: Vacuum-induced Autler-Townes splitting in a superconducting artificial atom
Source: arXiv:1705.11118 source file (2018-01-05)
Supplement: Supplementary file 1 [file Supplementary_materialsJan04.pdf]

# Supplementary materials for "Vacuum-induced Autler-Townes splitting in a superconducting artificial atom"

Z.H. Peng, J.H. Ding, Y. Zhou, L.L. Ying, Z. Wang, L. Zhou, L.M. Kuang, Yu-xi Liu, O. Astafiev, and J.S. Tsai

## S1. The device

Our device represents an alpha-loop flux qubit, fabricated by means of the electron-beam lithography with an aluminium shadow evaporation technique. An SEM image of the device is shown in Fig. S1 and was discussed in Ref. [1, 2]. It contains two loops and two Josephson junctions of 200×400 nm$^2$ size. The effective Josephson energy of each junction $E_J/h$ = 120 GHz and the junction capacitances $C_J$ = 4 fF. The alpha-loop is a SQUID with two Josephson junctions of 200×160 nm$^2$ each.

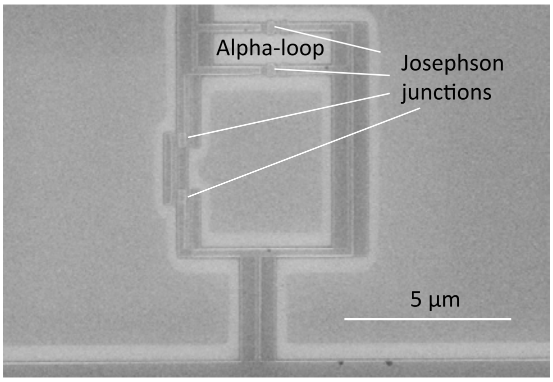


Figure S1. An SEM micrograph of our artificial atom of the alpha-loop qubit geometry.

## S2. Coupling between the open space and the resonator via the quantum system

Our artificial atom is capacitively coupled to the resonator and to the transmission line via capacitances $C_r \approx 2$ fF and $C_l \approx 4.8$ fF. Coupling between the two macroscopic systems and reflection from the quantum system has been discussed in Ref. [2]. We can estimate impedance between the resonator and the open line via the effective capacitance $C_{rl} = C_r\, C_l/(C_r + C_l) \approx 1.4$ fF. The effective impedance between the resonator and the open space from the side of the atom is Z = $1/(i\omega C_{rl}) \approx 10^4\ \Omega$ for $\omega/2\pi$=10GHz . However, this value is more appropriate to characterise two open lines as it was in Ref. [2]. In case of the resonator, it is more appropriate to compare $C_{rl}$ with the capacitance which defines loading loss (the capacitance between the resonator and CPW in Fig. 1(a)). The loaded capacitance for the photon decay rate

$\kappa/2\pi$ = 3.6 MHz is found to be $C_k$ = 13 fF, which is 10 times larger than the parasitic capacitances to the left hand side open line. The decoupling of the resonator from the left hand side transmission line is confirmed experimentally. The resonator line is invisible in Fig. 2(a, b) in the reflection spectrum away from the atomic resonances.

## S3. Reflection measurements and the concept of strong coupling of the system to the open line

Here we generalize the propagating wave reflection and define the strong coupling for the multi-level system, extending the discussion of Ref. [3]. Figure S3 exemplifies the three-level system with all transitions and level broadenings. For simplicity, we consider a weak driving regime (the driving amplitude $\Omega$ is much smaller than rates of incoherent processes) with a small detuning $\delta\omega = \omega - \omega_{jk}$ in respect to the resonance between two levels $|k\rangle$ and $|j\rangle$, with energy of $|j\rangle$ larger than $|k\rangle$, where {k,j}={g,e,f}. The general form of reflection coefficient in stationary conditions can be written as

$$r = 1 - \frac{\Gamma_{jk}\left(\rho_{kk} - \rho_{jj}\right)}{\lambda_{kj}\left(1 - i\delta\omega/\lambda_{kj}\right)}, \qquad \text{(S1)}$$

where $\Gamma_{jk}$ is the relaxation rate from the level $|j\rangle$ to $|k\rangle$, $\rho_{jj}$ and $\rho_{kk}$ are the level populations, $\lambda_{kj}$ is the decay rate of off-diagonal terms $\rho_{kj}$ and $\rho_{jk}$ of the atom density matrix. In the simple case of the two-level system, $\lambda_{kj}$ is the total dephasing rate. Let us start the analysis of reflection from a two-level system without pure dephasing. In such a case, $\Gamma_{eg}/2\lambda_{ge} = 1$ at $T = 0$ ($\rho_{gg} = 1$, $\rho_{ee} = 0$). And the absolute value of the reflection coefficient $|r|$ is always unity, however the phase of $r$ depends on $\delta\omega$. For the two-level system, we can define the strong coupling regime when the photon relaxation to the transmission line dominates comparing other incoherent processes, for example, $\lambda_{ge} \leq \Gamma_{eg}$. Particularly, when $\lambda_{ge} = \Gamma_{eg}$ and $\rho_{gg} = 1$, not less than 50% of photons are emitted to the line from the excited system.

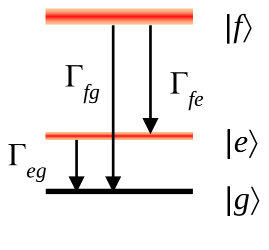


Figure S2. Schematics of the three-level system. The level broadening can be caused by the atomic relaxations and dephasing

The situation is different in case of a multi-level system. The first important consequence from Eq. (S1) is that for the three- and more level system even in an ideal situation in the absence of dephasing and non-radiative decay, the reflection still

can be less than 100% due to competition between the relaxation processes. For example, if the relaxation processes from the $|f\rangle$-level are $|f\rangle \to |g\rangle$ and $|f\rangle \to |e\rangle$, $(\Gamma_{fg} + \Gamma_{fe})/2=\lambda_{gf} < \Gamma_{fg}$.

Figure S3(a) shows the reflection from the lowest two levels ($|g\rangle \to |e\rangle$) of our system at frequency 11.45 GHz. The red curve is a fit of $A/(1-i\omega_{\rm eg}/\lambda_{eg})$ with $A = 0.75$. The plot proves strong coupling of our two-level system to the open transmission line from the right-hand side in Fig. 1(a). If we assume that $\rho_{ee} \approx 0$ then $\Gamma_{eg}/2\lambda_{ge} = 0.75$. Two conclusions are the dephasing rate is weak and the photon escape rate to the line with probability 75% and that is $\lambda_{ge} < \Gamma_{eg}$. Figure S3(b) shows a Lorentzian fit of $|(1 - r)/2|^2$. The peak width FWHM $\Delta\omega/2\pi = 19$ MHz ($= 2\lambda_{ge}$) at $\omega_{eg}/2\pi = 11.45$ GHz .

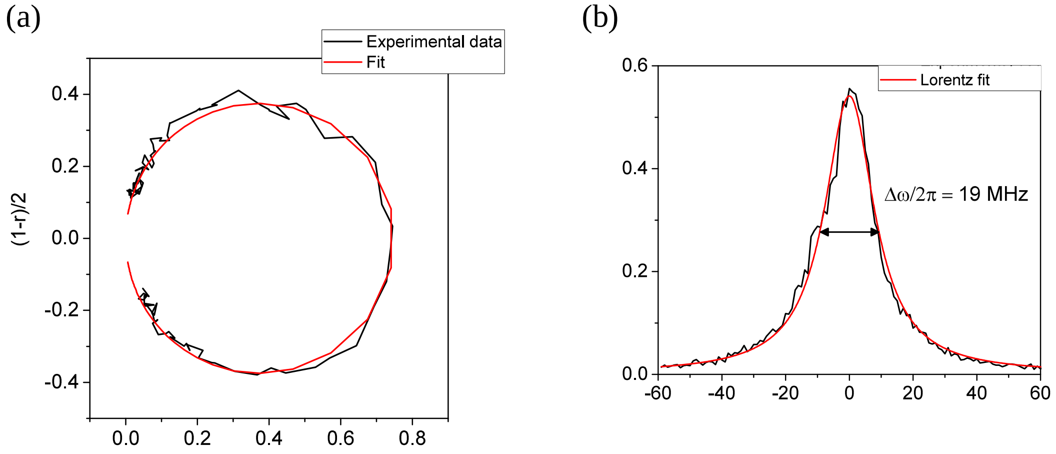


Figure S3. (a) A plot of $(r - 1)/2$ in real-imaginary coordinate of the two-level system ($|g\rangle \to |e\rangle$ transition). The red curve is the fit with amplitude 0.75. $|(1\text{-r})/2|^2$ fitted by Lorentzian by with FWHM $\Delta\omega/2\pi = 19$ MHz.

## S4. Reflection from the three-level system at a finite temperature

Similarly to the two-level system, we define the strong coupling for a multi-level system, when the photons predominantly escape to the open line. As it follows from Eq. (S1), at absolute zero temperature ($T = 0$) all levels are unpopulated except the ground state $|g\rangle$. Therefore, only transition from the ground state ($|g\rangle \leftrightarrow |e\rangle$ and $|g\rangle \leftrightarrow |f\rangle$) are visible and the transition from $|e\rangle$ state is not visible because $\rho_{\rm ee} = 0$ as it follows from Eq. (S1). At a finite temperature $T$, all populations are non-zero and the transition between excited states become visible. When temperature is low and the population is weak, the reflection in resonance ($\delta\omega = 0$) becomes $r_{fe} \approx 1 - \frac{\Gamma_{fe}}{\lambda_{ef}}\rho_{ee}$ and $\frac{1-r}{2} = \frac{\Gamma_{fe}}{2\lambda_{ef}}\rho_{ee}$. If we assume $\rho_{ff} \approx 0$, the population of the excited state is

$\rho_{ee} \approx \left[1+\exp\left(\hbar\omega_{eg}/k_B T\right)\right]^{-1}$. Figure S4 presents fitting of (1 – $r_{fe}$)/2 measured at different frequencies by $A/\left[1+\exp\left(\hbar\omega_{eg}/k_B T\right)\right]$ and we find the fitting parameters $A$ = 0.68 ($A=\Gamma_{fe}/2\lambda_{ef}$), $T$ = 0.075 K. Note that the extracted effective temperature in our system is a reasonable value [4, 5]. The $A$ value satisfy the condition of strong coupling. At the working point in the inset of Fig. 2(c), $|r|^2 = (1 - \rho_{ee}\,\Gamma_{fe}/\lambda_{ef})^2 \approx 0.78$, which is very close to the experimentally observed dips. We also find the population of the $|e\rangle$-level at the working point ($\omega_{eg}$ = 3.379 GHz) to be $\rho_{ee} \approx 0.1$.

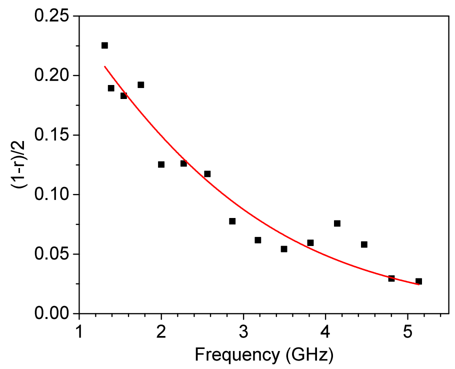


Figure S4. Thermal population of the $|e\rangle$-level measured extracted from the reflection at $|g\rangle \leftrightarrow |e\rangle$ transition (1-r)/2. The population is fitted by $A/\left[1+\exp\left(\hbar\omega_{eg}/k_B T\right)\right]$.

Now we briefly discuss the reflection between the ground and the second state. Figure 2(c) shows $(1-r)/2$ in resonance of the $|g\rangle \leftrightarrow |f\rangle$ transition ($|1-r|^2 \approx 0.7$) in a regime when $\Omega^2 \approx 2\,\lambda_{gf}\Gamma_{eg}$ (this is deduced from analysis of the charts of $r$ similar to Fig. S3). We find $\Gamma_{fg}/\lambda_{gf} \approx 0.24$ and $\lambda_{gf}/2\pi \approx 16$ MHz. In the absence of pure dephasing $\lambda_{gf} = \left(\Gamma_{fg}+\Gamma_{fe}\right)/2$ and $\Gamma_{fg} \approx 0.16\,\Gamma_{fe}$. The result is very reasonable because we expect suppression of relaxation at frequencies above 12 GHz – the upper cut-off frequency of the bandpass filter in our system. Such a relaxation rate is expected if the noise is suppressed by two or three times. The filter situated at the base temperature suppresses the quantum noise of 50-Ω-line resistor resulting in a weaker relaxation rate. This is also confirmed by suppression of the signal, when we are measuring the reflections at 12.2 GHz.

We also simulated the couplings and relaxation rates and the numbers, taking from the fits and analysis, are $\Gamma_{fg}/2\pi \approx$ 4MHz, $\Gamma_{fe}/2\pi \approx 25$ MHz, $\Gamma_{eg}/2\pi \approx 2$ MHz. The probing amplitude is found to be $\Omega/2\pi \approx 7$ MHz.

**References**


[1]. A. Fedorov et al., Phys. Rev. Lett. **105**, 060503(2010).

[2]. Z. H. Peng et al., Nat. Commun. **7**, 12588 (2016).

[3]. O. Astafiev et al., Science **327**, 840 (2010).

[4]. K. Geerlings et al., Phys. Rev. Lett. **110**, 120501 (2013).

[5]. X. Y. Jin et al., Phys. Rev. Lett. **114**, 240501 (2015).
